# Supplementary material for: Deep Learning in Asset Pricing
Source: arXiv:1904.00745 source file (2021-08-11)
Supplement: Supplementary file 1 [file Internetappendix.pdf]

# **Internet Appendix for “Deep Learning in Asset Pricing”**

Luyang Chen, Markus Pelger and Jason Zhu<sup>1</sup>

## **Abstract**

This Internet Appendix provides additional tables and figures supporting the main text. Among others it includes the SDF structure as a function of additional characteristics and pricing results for additional portfolio sorts.

## **IA.A. Overview**

The Internet Appendix collects multiple robustness results that support the results in the main text. Section IA.B shows that the results are robust to the normalization of the SDF and the model performance for large cap stocks. Section IA.C collects the predictive performance results for the FFN, EN and LS model. In Section IA.D we provide the asset pricing results for additional characteristic sorted portfolios. Section IA.E shows the functional form of different SDFs conditioned on univariate or multiple characteristics.

---

<sup>1</sup>Citation format: Chen, Luyang, Pelger, Markus and Zhu, Jason, Internet Appendix for “Deep Learning in Asset Pricing”.

## IA.B. Robustness Results

**Table IA.I** SDF Factor Portfolio Performance without Normalized Weights

| Model | SR    |       |      | Max Loss |       |       | Max Drawdown |       |      |
|-------|-------|-------|------|----------|-------|-------|--------------|-------|------|
|       | Train | Valid | Test | Train    | Valid | Test  | Train        | Valid | Test |
| LS    | 1.82  | 0.57  | 0.41 | -1.54    | -1.96 | -5.13 | 1            | 3     | 4    |
| EN    | 1.28  | 1.13  | 0.47 | -2.20    | -1.82 | -5.77 | 1            | 3     | 5    |
| FFN   | 0.48  | 0.42  | 0.47 | -4.60    | -4.72 | -3.28 | 6            | 3     | 5    |
| GAN   | 3.21  | 1.45  | 0.72 | 0.18     | -0.27 | -5.95 | 0            | 1     | 5    |

Sharpe Ratio, maximum 1-month loss and maximum drawdown of the SDF factor portfolios.

**Table IA.II** SDF Factor Risk Measures for Large Market Cap Stocks

| Model                                   | SR    |       |       | Max Loss |       |       | Max Drawdown |       |      |
|-----------------------------------------|-------|-------|-------|----------|-------|-------|--------------|-------|------|
|                                         | Train | Valid | Test  | Train    | Valid | Test  | Train        | Valid | Test |
| Size $\geq 0.001\%$ of total market cap |       |       |       |          |       |       |              |       |      |
| LS                                      | 1.44  | 0.31  | 0.13  | -3.07    | -2.19 | -4.59 | 1            | 3     | 7    |
| EN                                      | 0.93  | 0.56  | 0.15  | -3.00    | -2.45 | -4.82 | 2            | 3     | 5    |
| FFN                                     | 0.42  | 0.20  | 0.30  | -3.89    | -4.66 | -4.33 | 6            | 4     | 5    |
| GAN                                     | 2.32  | 1.09  | 0.41  | -1.17    | -1.14 | -4.84 | 1            | 1     | 5    |
| Size $\geq 0.01\%$ of total market cap  |       |       |       |          |       |       |              |       |      |
| LS                                      | 0.32  | -0.11 | -0.06 | -3.11    | -1.82 | -3.67 | 4            | 5     | 7    |
| EN                                      | 0.37  | 0.26  | 0.23  | -4.44    | -2.67 | -4.66 | 4            | 3     | 7    |
| FFN                                     | 0.32  | 0.17  | 0.24  | -3.30    | -4.53 | -5.08 | 7            | 5     | 5    |
| GAN                                     | 0.97  | 0.54  | 0.26  | -6.91    | -1.36 | -5.01 | 2            | 2     | 7    |

Sharpe Ratio, maximum 1-month loss and maximum drawdown of the SDF factor portfolios. The model is evaluated on stocks with market capitalization larger than 0.01% or 0.001% of the total market capitalization.

## IA.C. Predictive Portfolios

**Figure IA.1.** Equally Weighted  $\beta$  Sorted Decile Portfolios with FFN

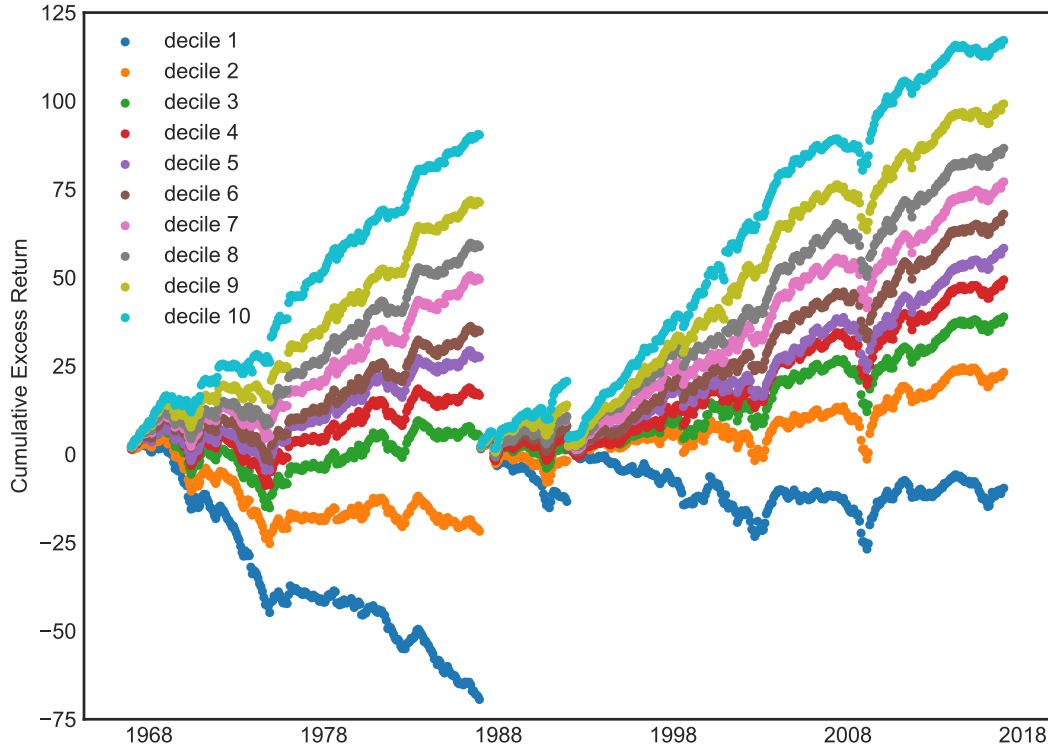

Cumulative excess return of decile sorted portfolios based on the risk loadings  $\beta$  for FFN. The first portfolio is based on the smallest decile of risk loadings, while the last decile portfolio is constructed with the largest loading decile. Within each decile the stocks are equally weighted.

**Figure IA.2.** Value Weighted  $\beta$  Sorted Decile Portfolios with FFN

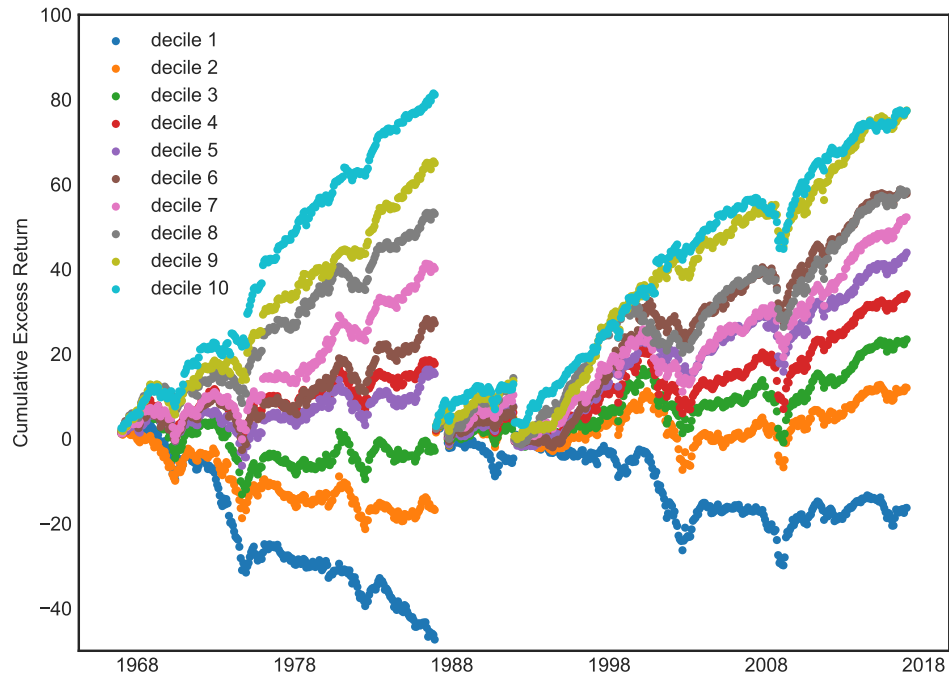

Cumulative excess return of decile sorted portfolios based on the risk loadings  $\beta$  for FFN. The first portfolio is based on the smallest decile of risk loadings, while the last decile portfolio is constructed with the largest loading decile. Within each decile the stocks are value weighted.

**Figure IA.3.** Equally Weighted  $\beta$  Sorted Decile Portfolios with EN

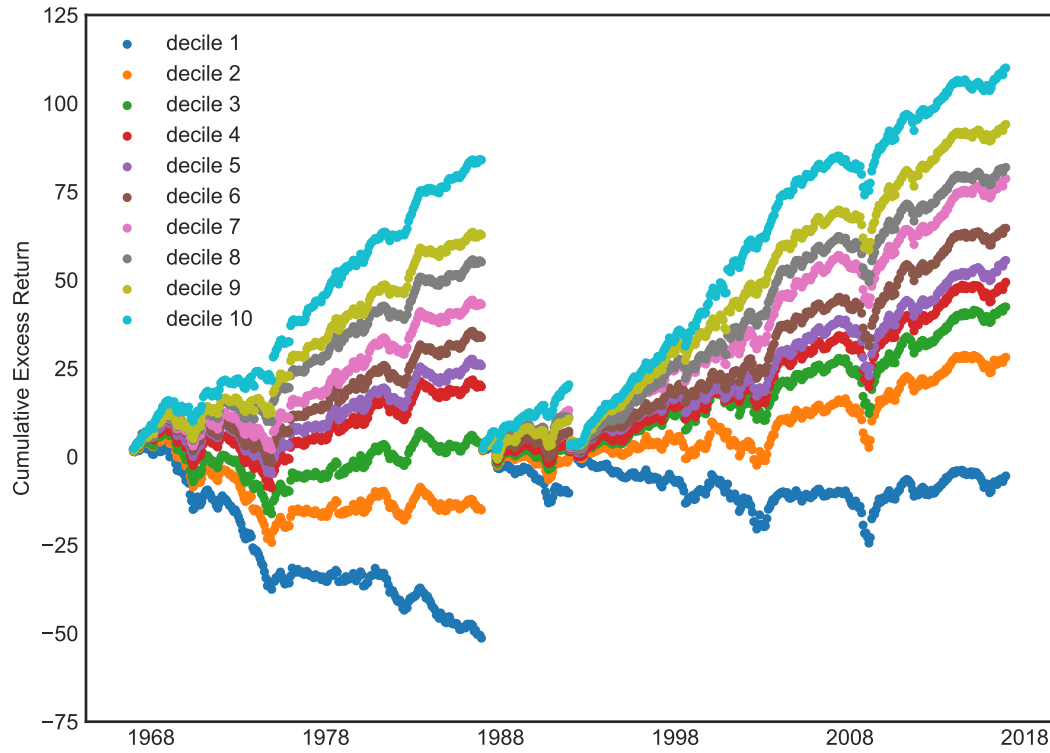

Cumulative excess return of decile sorted portfolios based on the risk loadings  $\beta$  for EN. The first portfolio is based on the smallest decile of risk loadings, while the last decile portfolio is constructed with the largest loading decile. Within each decile the stocks are equally weighted.

**Figure IA.4.** Value Weighted  $\beta$  Sorted Decile Portfolios with EN

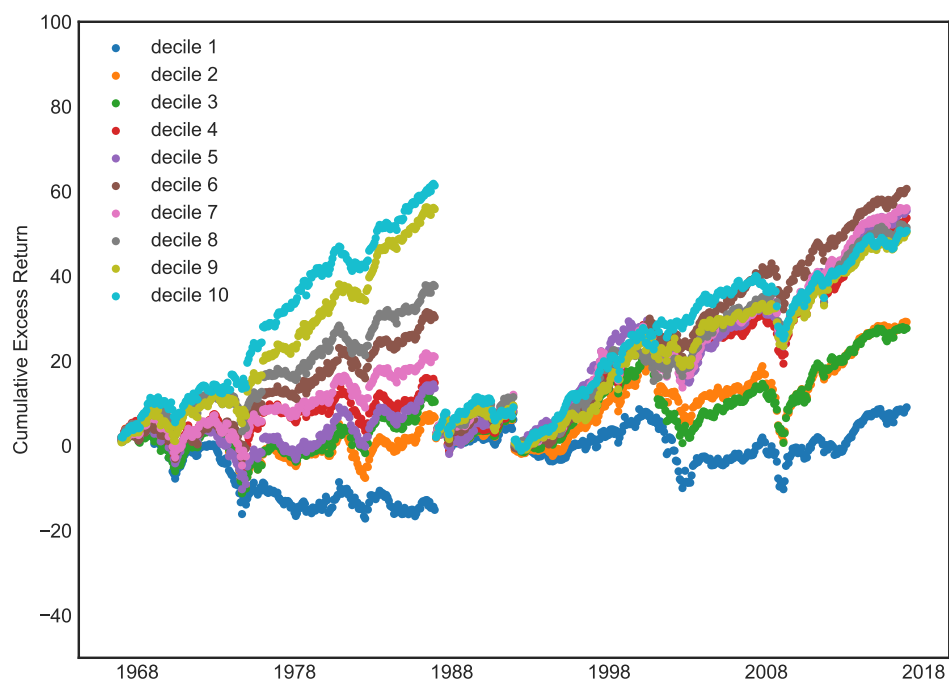

Cumulative excess return of decile sorted portfolios based on the risk loadings  $\beta$  for EN. The first portfolio is based on the smallest decile of risk loadings, while the last decile portfolio is constructed with the largest loading decile. Within each decile the stocks are value weighted.

**Figure IA.5.** Equally Weighted  $\beta$  Sorted Decile Portfolios with LS

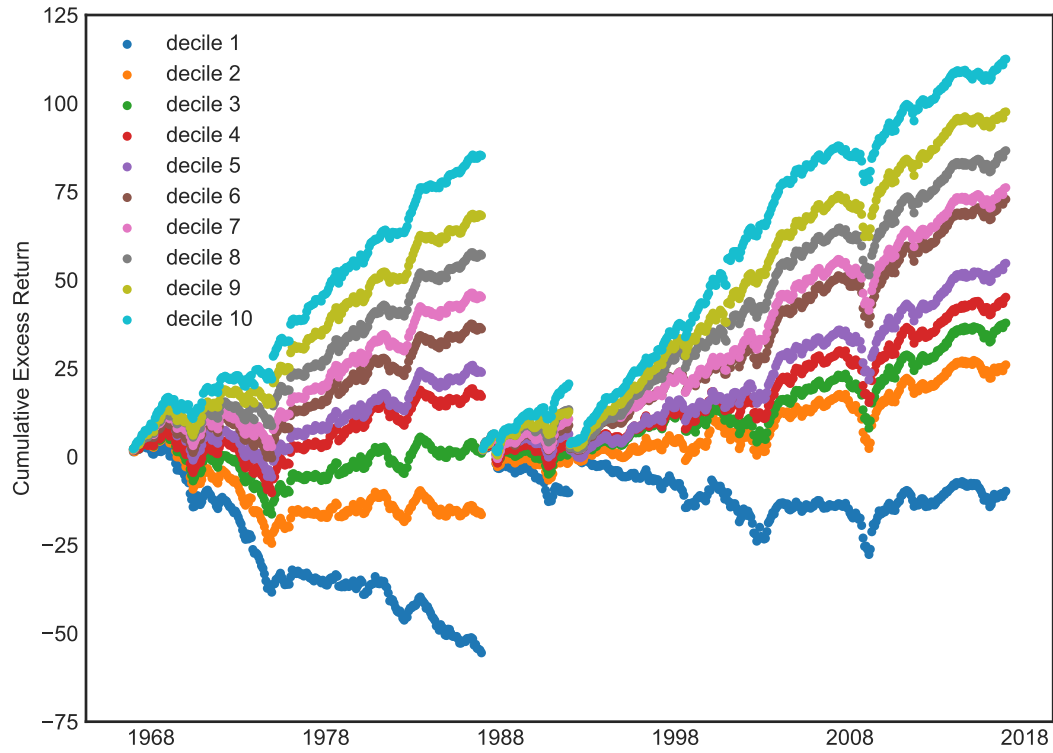

Cumulative excess return of decile sorted portfolios based on the risk loadings  $\beta$  for LS. The first portfolio is based on the smallest decile of risk loadings, while the last decile portfolio is constructed with the largest loading decile. Within each decile the stocks are equally weighted.

**Figure IA.6.** Value Weighted  $\beta$  Sorted Decile Portfolios with LS

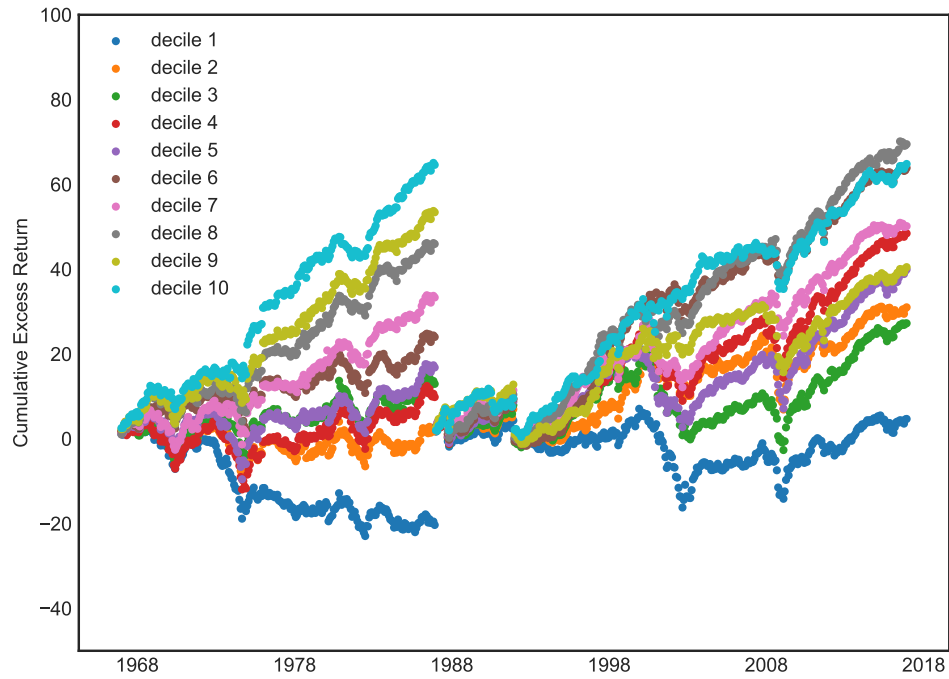

Cumulative excess return of decile sorted portfolios based on the risk loadings  $\beta$  for LS. The first portfolio is based on the smallest decile of risk loadings, while the last decile portfolio is constructed with the largest loading decile. Within each decile the stocks are value weighted.



## IA.D. Portfolio Pricing

**Table IA.III** Explained Variation and Pricing Errors for Size and Dividend Yield Sorted Portfolios

|     |     | EN                  | FFN  | GAN  |  | EN                    | FFN   | GAN   |
|-----|-----|---------------------|------|------|--|-----------------------|-------|-------|
| LME | D2P | Explained Variation |      |      |  | Alpha                 |       |       |
| 1   | 1   | 0.82                | 0.78 | 0.83 |  | -0.01                 | -0.01 | -0.02 |
| 1   | 2   | 0.79                | 0.72 | 0.78 |  | 0.01                  | 0.01  | -0.01 |
| 1   | 3   | 0.74                | 0.71 | 0.77 |  | 0.04                  | 0.02  | -0.00 |
| 1   | 4   | 0.29                | 0.30 | 0.31 |  | 0.09                  | 0.04  | 0.07  |
| 1   | 5   | 0.21                | 0.13 | 0.44 |  | -0.10                 | -0.11 | -0.04 |
| 2   | 1   | 0.82                | 0.51 | 0.83 |  | -0.03                 | 0.06  | -0.01 |
| 2   | 2   | 0.81                | 0.56 | 0.85 |  | 0.01                  | 0.08  | 0.01  |
| 2   | 3   | 0.72                | 0.54 | 0.78 |  | -0.01                 | 0.05  | -0.01 |
| 2   | 4   | 0.61                | 0.52 | 0.60 |  | -0.04                 | -0.03 | -0.07 |
| 2   | 5   | 0.51                | 0.58 | 0.67 |  | -0.07                 | -0.06 | -0.03 |
| 3   | 1   | 0.73                | 0.46 | 0.81 |  | 0.09                  | 0.15  | 0.06  |
| 3   | 2   | 0.76                | 0.54 | 0.84 |  | 0.04                  | 0.11  | 0.02  |
| 3   | 3   | 0.70                | 0.51 | 0.83 |  | 0.09                  | 0.15  | 0.06  |
| 3   | 4   | 0.77                | 0.69 | 0.83 |  | 0.05                  | 0.07  | 0.02  |
| 3   | 5   | 0.67                | 0.70 | 0.70 |  | -0.05                 | -0.04 | -0.03 |
| 4   | 1   | 0.62                | 0.47 | 0.80 |  | 0.12                  | 0.14  | 0.04  |
| 4   | 2   | 0.67                | 0.58 | 0.83 |  | 0.08                  | 0.09  | 0.01  |
| 4   | 3   | 0.59                | 0.52 | 0.79 |  | 0.10                  | 0.10  | 0.02  |
| 4   | 4   | 0.77                | 0.78 | 0.78 |  | 0.03                  | -0.00 | -0.02 |
| 4   | 5   | 0.56                | 0.54 | 0.54 |  | -0.07                 | -0.09 | -0.07 |
| 5   | 1   | 0.15                | 0.35 | 0.53 |  | 0.11                  | 0.07  | 0.01  |
| 5   | 2   | 0.23                | 0.39 | 0.60 |  | 0.09                  | 0.05  | 0.00  |
| 5   | 3   | 0.23                | 0.21 | 0.51 |  | 0.03                  | -0.05 | -0.06 |
| 5   | 4   | 0.40                | 0.22 | 0.36 |  | -0.03                 | -0.09 | -0.06 |
| 5   | 5   | 0.36                | 0.38 | 0.43 |  | -0.00                 | -0.06 | -0.03 |
|     |     | Explained Variation |      |      |  | Cross-Sectional $R^2$ |       |       |
| All |     | 0.58                | 0.50 | 0.67 |  | 0.89                  | 0.84  | 0.96  |

Out-of-sample explained variation and pricing errors for double sorted portfolios based on Size (LME) and Dividend Yield (D2P).

**Table IA.IV** Explained Variation and Pricing Errors for Standard Unexplained Volume Sorted Portfolios

| SUV    | EN                  | FFN  | GAN  |  | EN                    | FFN   | GAN   |
|--------|---------------------|------|------|--|-----------------------|-------|-------|
| Decile | Explained Variation |      |      |  | Alpha                 |       |       |
| 1      | -0.22               | 0.50 | 0.78 |  | 0.28                  | 0.00  | -0.06 |
| 2      | -0.03               | 0.64 | 0.82 |  | 0.33                  | 0.10  | 0.03  |
| 3      | 0.11                | 0.69 | 0.80 |  | 0.26                  | 0.06  | 0.02  |
| 4      | 0.28                | 0.71 | 0.80 |  | 0.21                  | 0.03  | -0.01 |
| 5      | 0.49                | 0.79 | 0.83 |  | 0.16                  | 0.02  | 0.01  |
| 6      | 0.58                | 0.84 | 0.87 |  | 0.10                  | -0.04 | -0.04 |
| 7      | 0.72                | 0.84 | 0.86 |  | 0.11                  | 0.00  | 0.03  |
| 8      | 0.78                | 0.82 | 0.85 |  | 0.03                  | -0.01 | 0.01  |
| 9      | 0.76                | 0.78 | 0.83 |  | -0.03                 | -0.09 | -0.02 |
| 10     | 0.76                | 0.83 | 0.85 |  | -0.13                 | -0.06 | -0.00 |
|        | Explained Variation |      |      |  | Cross-Sectional $R^2$ |       |       |
| All    | 0.42                | 0.75 | 0.83 |  | 0.64                  | 0.97  | 0.99  |

Out-of-sample explained variation and pricing errors for decile sorted portfolios based on Standard Unexplained Volume (SUV).

**Table IA.V** Explained Variation and Pricing Errors for Net Operating Assets Sorted Portfolios

| NOA    | EN                  | FFN  | GAN  |  | EN                    | FFN   | GAN   |
|--------|---------------------|------|------|--|-----------------------|-------|-------|
| Decile | Explained Variation |      |      |  | Alpha                 |       |       |
| 1      | 0.41                | 0.55 | 0.66 |  | 0.17                  | 0.10  | 0.09  |
| 2      | 0.57                | 0.72 | 0.80 |  | 0.05                  | -0.01 | 0.04  |
| 3      | 0.58                | 0.79 | 0.84 |  | -0.06                 | -0.07 | -0.03 |
| 4      | 0.69                | 0.76 | 0.78 |  | 0.02                  | 0.01  | 0.05  |
| 5      | 0.73                | 0.75 | 0.77 |  | -0.03                 | -0.04 | 0.00  |
| 6      | 0.64                | 0.75 | 0.75 |  | 0.06                  | 0.03  | 0.05  |
| 7      | 0.72                | 0.82 | 0.83 |  | 0.02                  | -0.01 | -0.00 |
| 8      | 0.67                | 0.75 | 0.84 |  | -0.08                 | -0.12 | -0.13 |
| 9      | 0.66                | 0.79 | 0.85 |  | 0.10                  | 0.07  | 0.02  |
| 10     | 0.43                | 0.47 | 0.75 |  | -0.04                 | -0.06 | -0.15 |
|        | Explained Variation |      |      |  | Cross-Sectional $R^2$ |       |       |
| All    | 0.58                | 0.69 | 0.78 |  | 0.94                  | 0.96  | 0.95  |

Out-of-sample explained variation and pricing errors for decile sorted portfolios based on Net Operating Assets (NOA).

## IA.E. SDF Structure

### IA.E.1. One-Dimensional Relationship

**Figure IA.7.** SDF weight  $\omega$  as a Function of Covariates for GAN

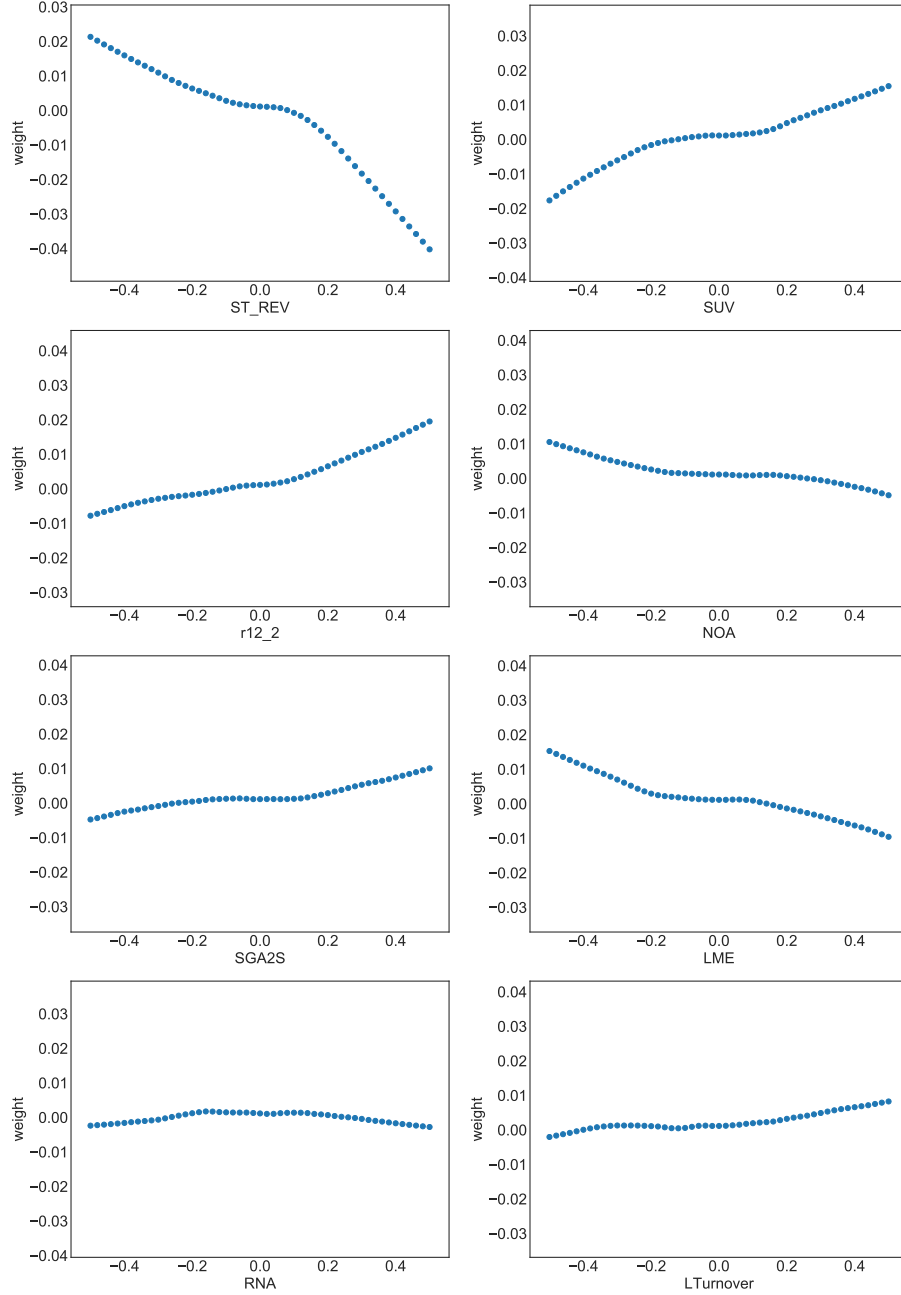

SDF weight  $\omega$  as a one-dimensional function of covariates keeping the other covariates at their mean level. The covariates are Short-Term Reversal (ST.REV), Standard Unexplained Volume (SUV), Momentum (r12.2), Net Operating Assets (NOA), Selling, General and Administrative Expenses to Sales (SGA2S), Size (LME), Return on Net Operating Assets (RNA) and Turnover (LTurnover).

**Figure IA.8.** SDF weight  $\omega$  as a Function of Covariates for FFN

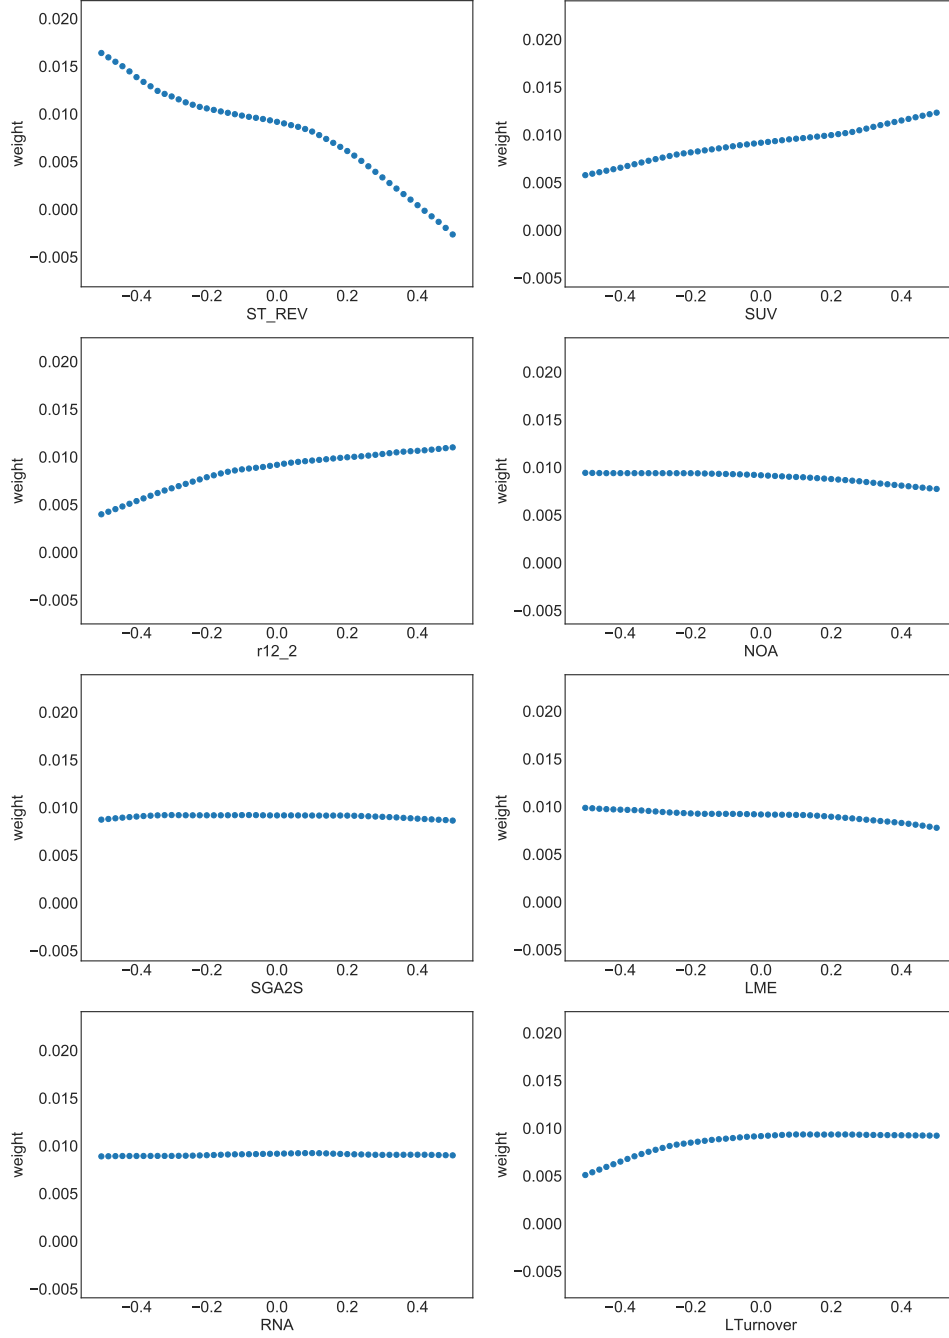

SDF weight  $\omega$  as a one-dimensional function of covariates keeping the other covariates at their mean level. The covariates are Short-Term Reversal (ST\_REV), Standard Unexplained Volume (SUV), Momentum (r12.2), Net Operating Assets (NOA), Selling, General and Administrative Expenses to Sales (SGA2S), Size (LME), Return on Net Operating Assets (RNA) and Turnover (LTurnover).

**Figure IA.9.** SDF weight  $\omega$  as a Function of Covariates for EN

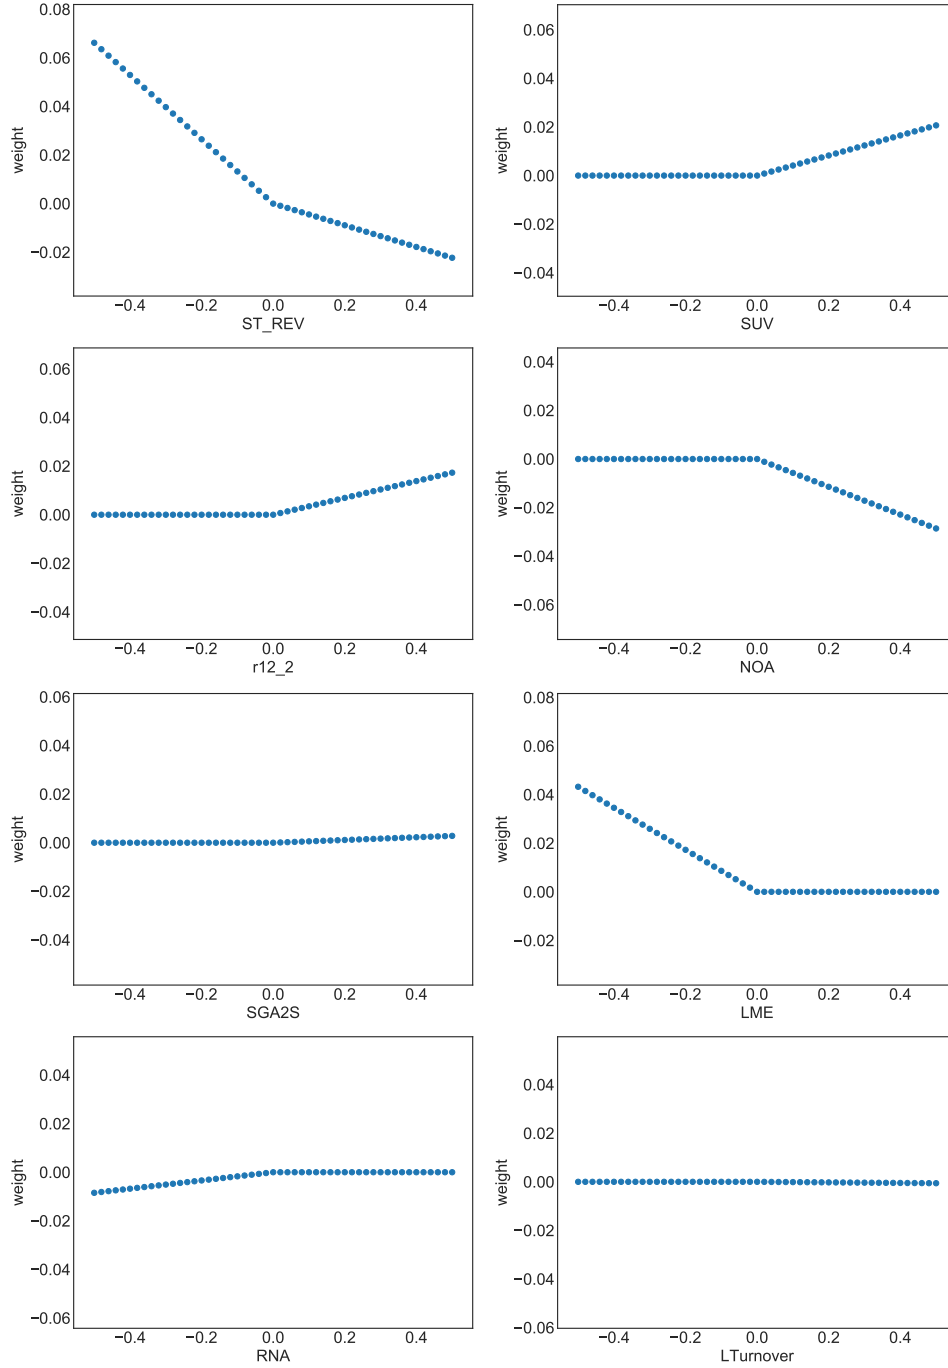

SDF weight  $\omega$  as a one-dimensional function of covariates keeping the other covariates at their mean level. The covariates are Short-Term Reversal (ST.REV), Standard Unexplained Volume (SUV), Momentum (r12.2), Net Operating Assets (NOA), Selling, General and Administrative Expenses to Sales (SGA2S), Size (LME), Return on Net Operating Assets (RNA) and Turnover (LTurnover).

**Figure IA.10.** SDF weight  $\omega$  as a Function of Covariates for LS

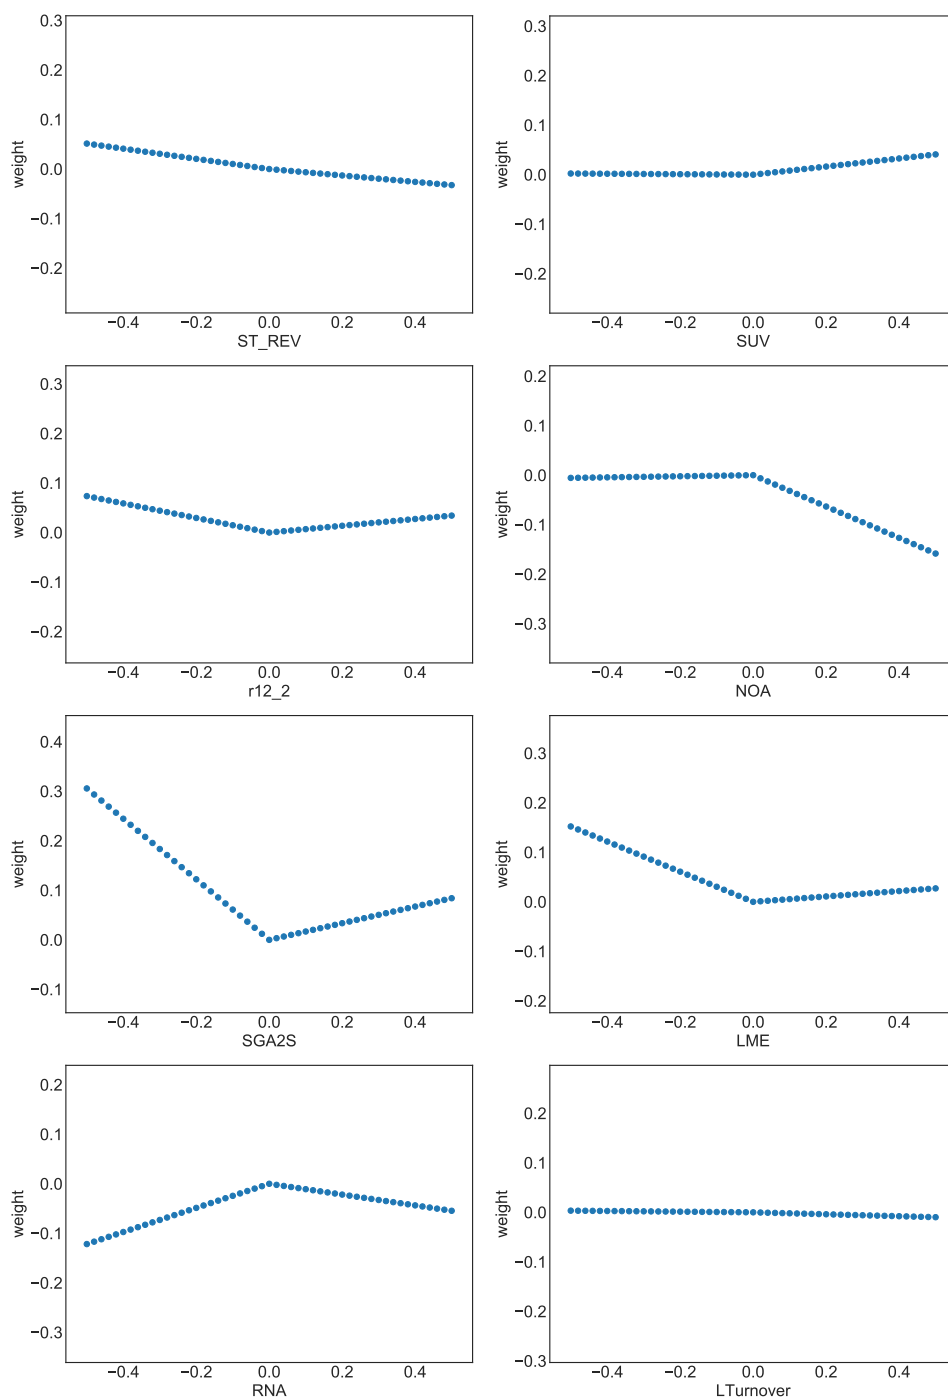

SDF weight  $\omega$  as a one-dimensional function of covariates keeping the other covariates at their mean level. The covariates are Short-Term Reversal (ST\_REV), Standard Unexplained Volume (SUV), Momentum (r12\_2), Net Operating Assets (NOA), Selling, General and Administrative Expenses to Sales (SGA2S), Size (LME), Return on Net Operating Assets (RNA) and Turnover (LTurnover).

IA.E.2. *Interaction between Characteristics*

**Figure IA.11.** Interaction between Size (LME) and Dividend Yield (D2P)

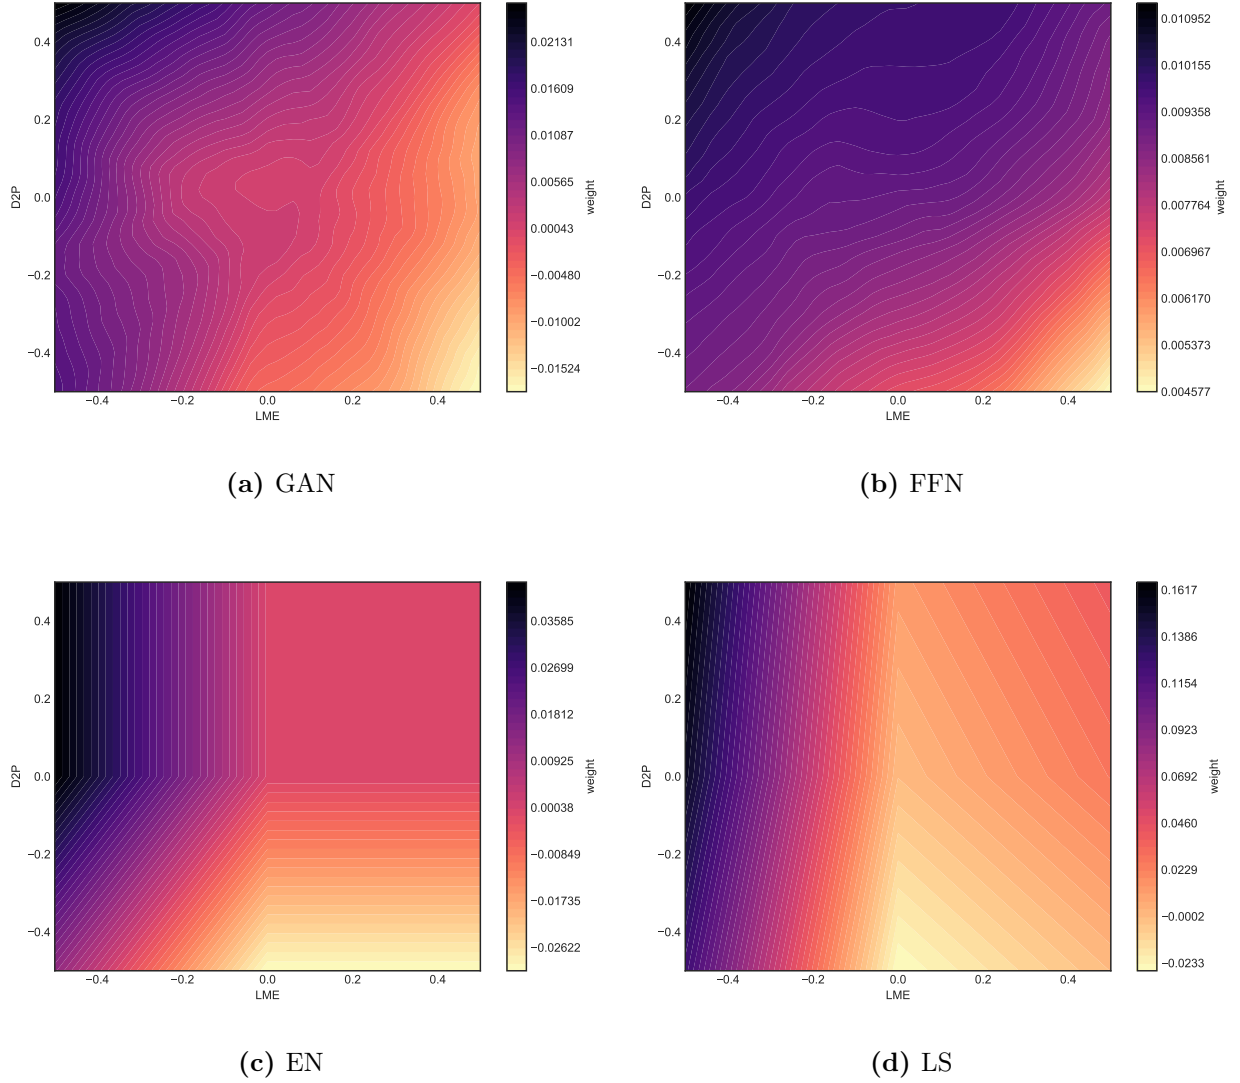

SDF weight  $\omega$  as a two-dimensional function of covariates keeping the other covariates at their mean level. The two covariates are Size (LME) and Dividend Yield (D2P)

**Figure IA.12.** Interaction between Size (LME), Book to Dividend Yield (D2P) and Short-Term Reversal (ST\_REV)

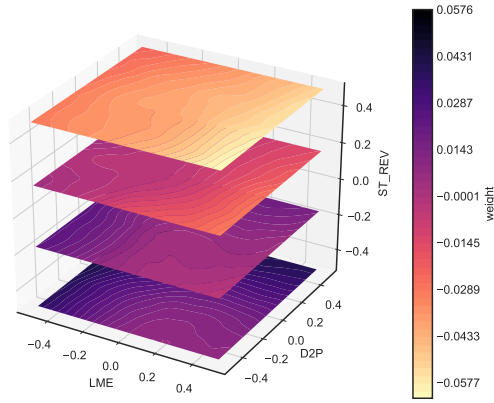

(a) GAN

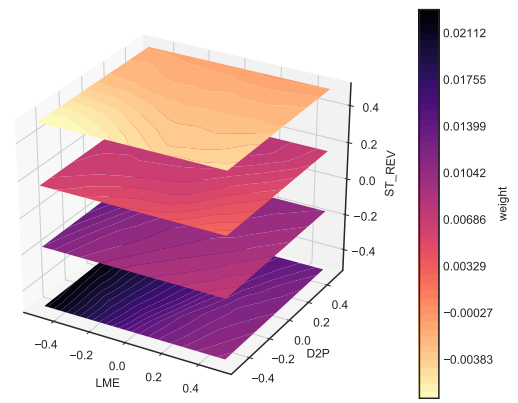

(b) FFN

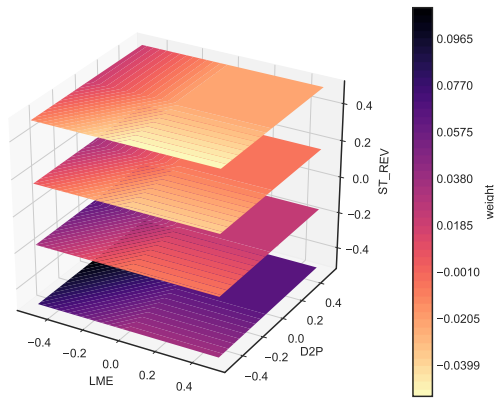

(c) EN

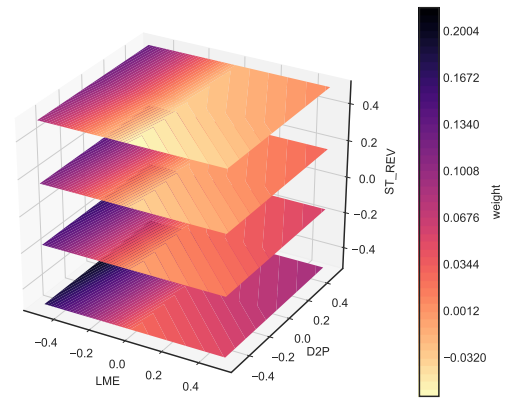

(d) LS

SDF weight  $\omega$  as a three-dimensional function of covariates keeping the other covariates at their mean level. The three covariates are Size (LME), Book to Dividend Yield (D2P) and Short-Term Reversal (ST\_REV).



**Figure IA.13.** Interaction between Size (LME) and Dividend Yield (D2P)

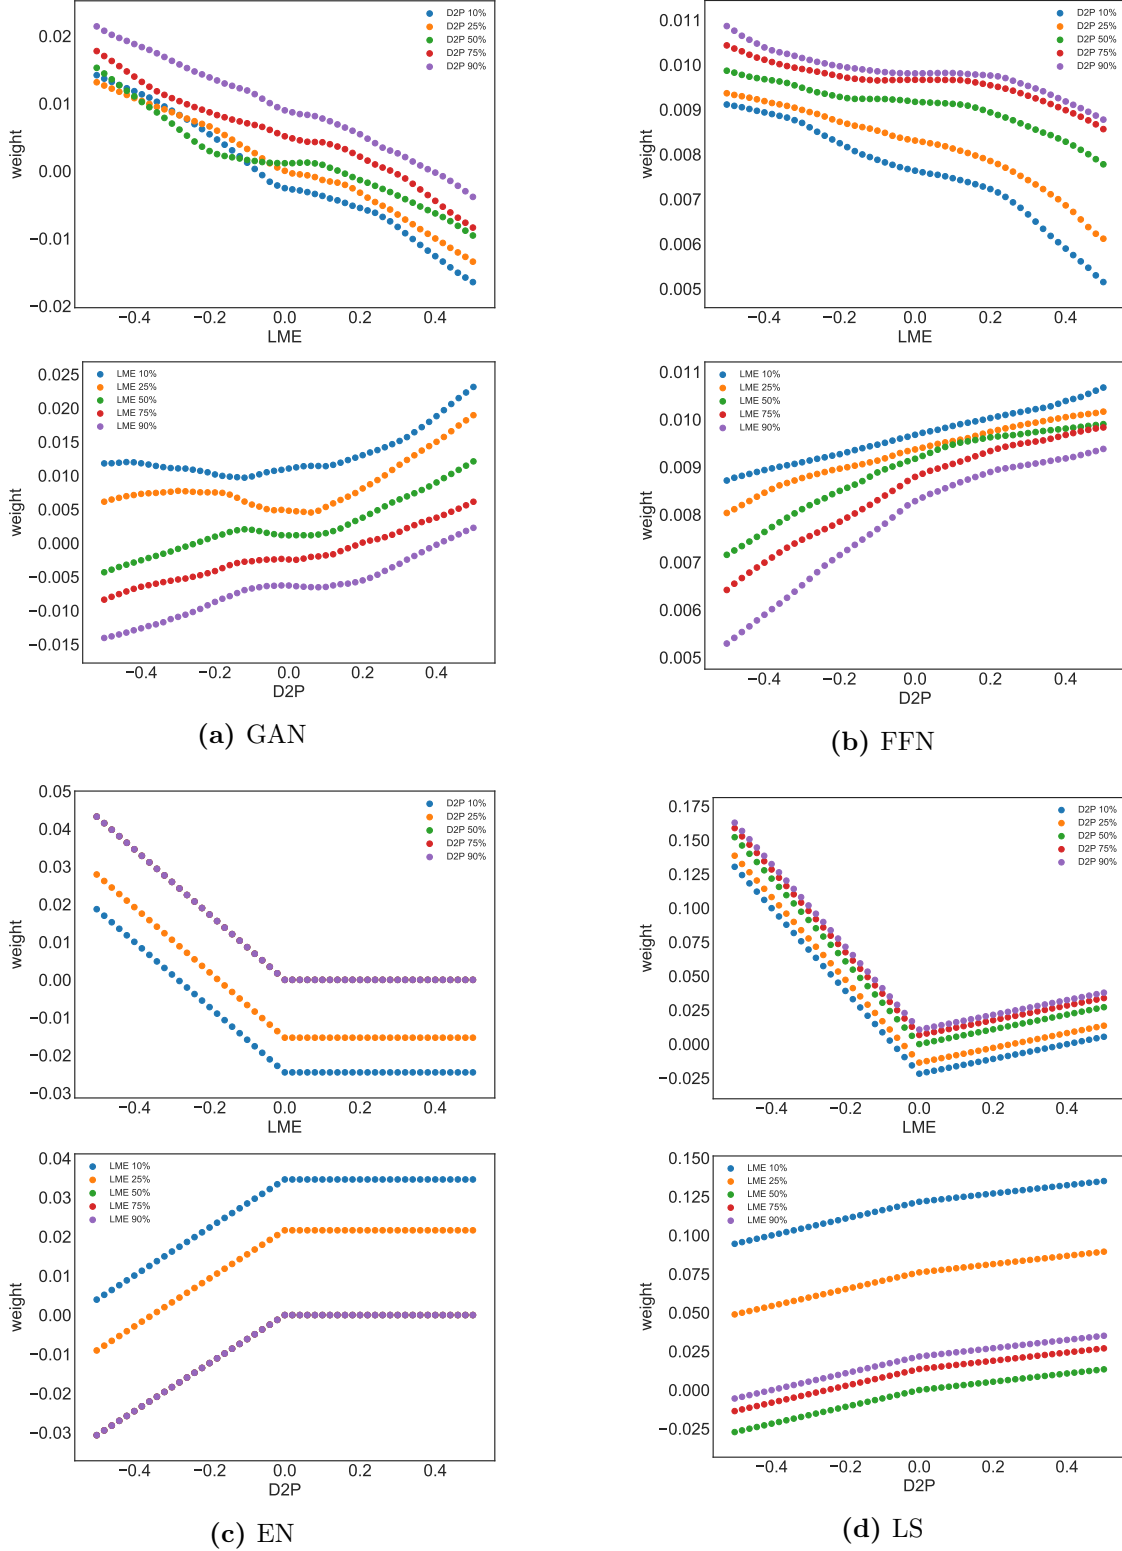

SDF weight  $\omega$  as a two-dimensional function of covariates keeping the other covariates at their mean level. The two covariates are Size (LME) and Dividend Yield (D2P)

**Figure IA.14.** SDF weight  $\omega$  as a Function of Covariates for FFN

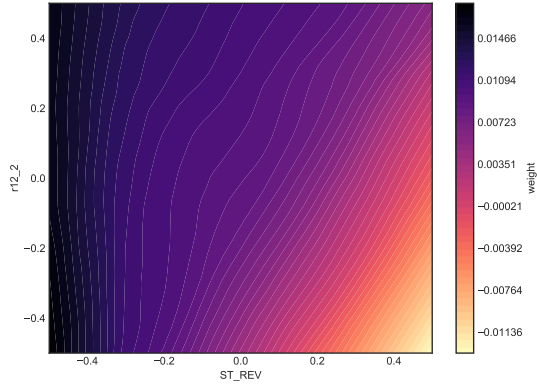

**(a)** Interaction between Short-Term Reversal (ST\_REV) and Momentum (r12\_2)

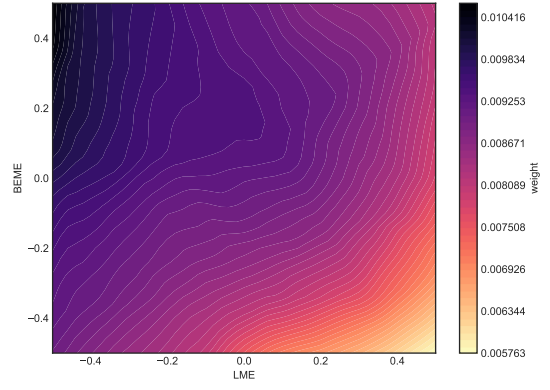

**(b)** Interaction between Size (LME) and Book to Market Ratio (BEME)

**Figure IA.15.** SDF weight  $\omega$  as a Function of Covariates for FFN

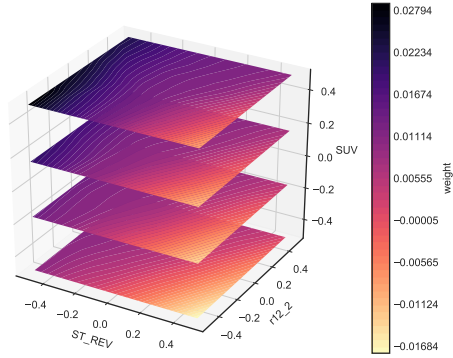

**(a)** Interaction between Short-Term Reversal (ST\_REV), Momentum (r12\_2) and Standard Unexplained Volume (SUV)

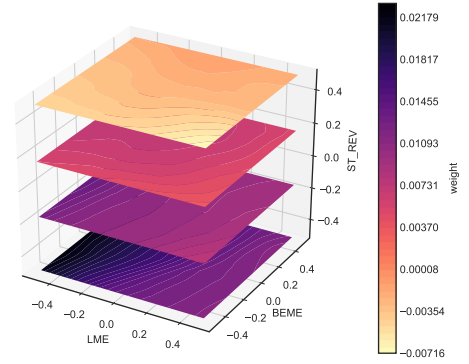

**(b)** Interaction between Size (LME), Book to Market Ratio (BEME) and Short-Term Reversal (ST\_REV)

**Figure IA.16.** SDF weight  $\omega$  as a Function of Covariates for EN

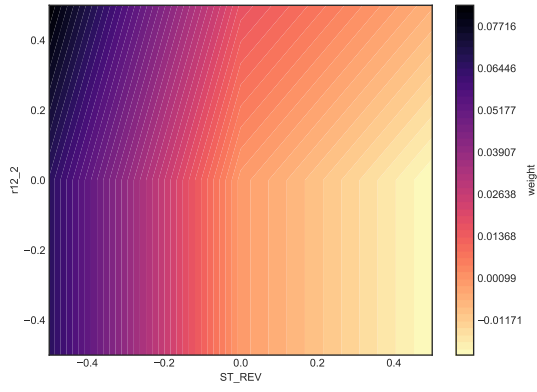

**(a)** Interaction between Short-Term Reversal (ST\_REV) and Momentum (r12\_2)

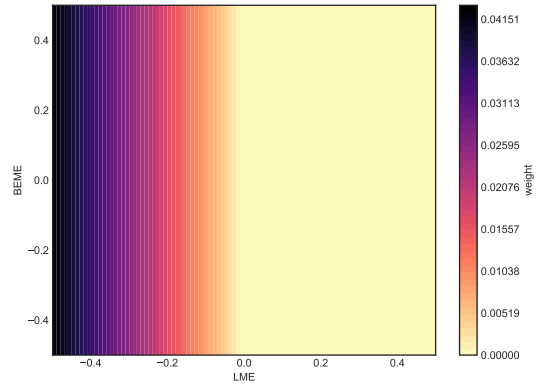

**(b)** Interaction between Size (LME) and Book to Market Ratio (BEME)

**Figure IA.17.** SDF weight  $\omega$  as a Function of Covariates for EN

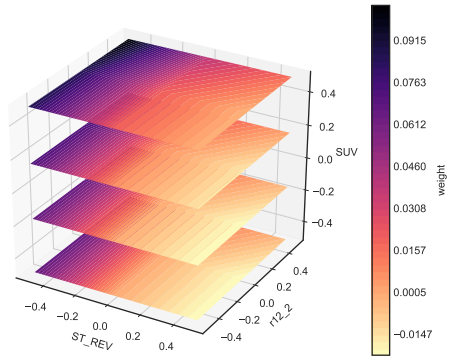

**(a)** Interaction between Short-Term Reversal (ST\_REV), Momentum (r12\_2) and Standard Unexplained Volume (SUV)

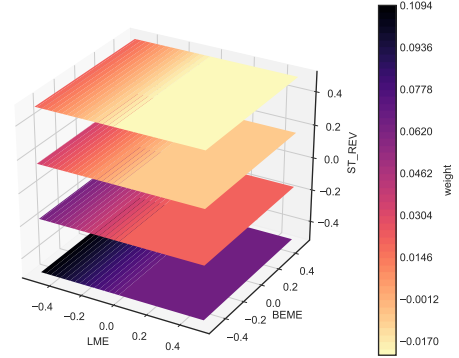

**(b)** Interaction between Size (LME), Book to Market Ratio (BEME) and Short-Term Reversal (ST\_REV)

**Figure IA.18.** SDF weight  $\omega$  as a Function of Covariates for LS

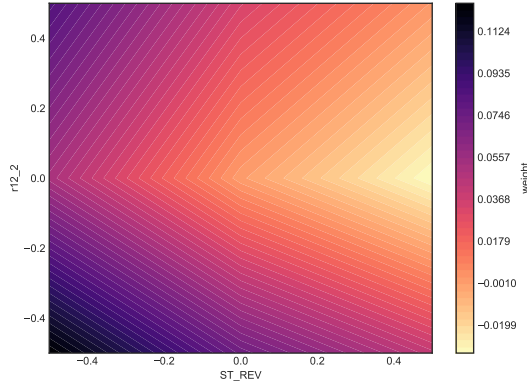

**(a)** Interaction between Short-Term Reversal (ST\_REV) and Momentum (r12\_2)

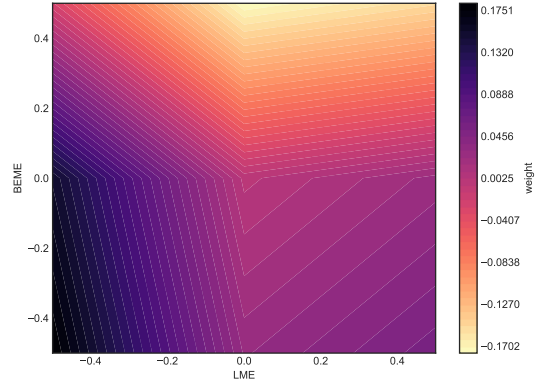

**(b)** Interaction between Size (LME) and Book to Market Ratio (BEME)

**Figure IA.19.** SDF weight  $\omega$  as a Function of Covariates for LS

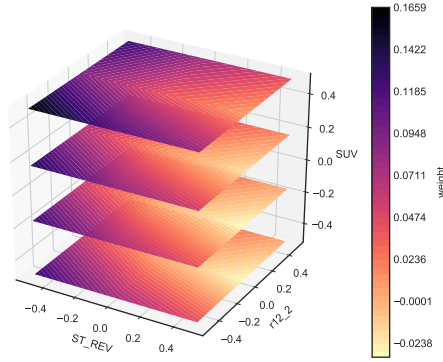

**(a)** Interaction between Short-Term Reversal (ST\_REV), Momentum (r12\_2) and Standard Unexplained Volume (SUV)

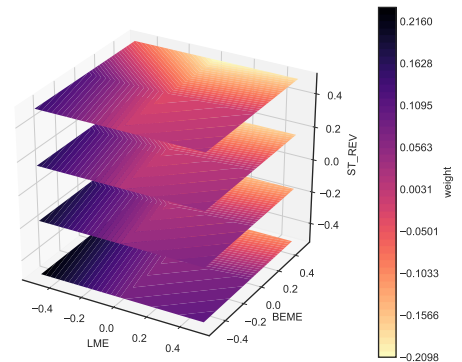

**(b)** Interaction between Size (LME), Book to Market Ratio (BEME) and Short-Term Reversal (ST\_REV)
